# Supplementary material for: A Mathematical Modeling Study of COVID-19 With Reference to Immigration from Urban to Rural Population
Source: arXiv:2205.05618 source file (2022-05-06)
Supplement: Supplementary file 1 [file AppendixA.tex]

\chapter{MATLAB Codes}

In the appendix, we give the MATLAB codes for the each of the plots in the thesis.

\section{Chapter 7 : Numerical Simulations}
This section includes the MATLAB codes of plots of chapter 7.

\noindent
\\
\underline{\textbf{\large{Figure \ref{df_gas_two_fig} (a)}}}\textbf{\large{ : }} The parameter values are from table \ref{df_gas_parameters}.

\begin{lstlisting}

% - - - - - - - Finding the value of Ro - - - - - - - %

global alpha beta Lamda mu tetha eps u1 u2 d m gamma R0

alpha = 0.95;
beta =  0.045;
Lamda = 2;
mu = 0.05;
tetha = 0.3;
eps = 0.03;
u1 = 0.1;
u2 = 0.1;
d = 0.01;
m = 0.1;
gamma = 0.01;

R0 = (eps*beta*Lamda)/((mu+tetha)*(mu+eps+u1)*(mu+d+gamma));

% - - - - - - - - - - - - - - - - - - - - - - - - - - - %
\end{lstlisting}

\newpage

\begin{lstlisting}
% - - - - - Defining the system as a function - - - - - %

function dx = type3(t,x)

global alpha beta Lamda mu tetha eps u1 u2 d m gamma

dx = zeros(3,1);
dx(1) = Lamda-(beta*x(1)*x(3)/(1+m*(x(3))))-mu*x(1)-tetha*x(1);
dx(2) = (beta*x(1)*x(3)/(1+m*(x(3)))) -(mu+eps+u1)*x(2);
dx(3) = eps*x(2)-(mu+d+gamma)*x(3) ...
        -(u2*(x(3)^2)/(1+alpha*(x(3)^2)));

end

% - - - - - - - - - - - - - - - - - - - - - - - - - - - %

% - - - - - - Plotting the solution curves - - - - - - %

global alpha beta Lamda mu tetha eps u1 u2 d m gamma R0

S_df = Lamda/(mu+tetha) % disease free equilibrium %

S_0 = 10;               % Initial conditions %
E_0 = 0;                
I_0 = 2;
x0 = [S_0 E_0 I_0];

tspan = 0 : 0.1 : 3000;
[tsol,xsol] = ode45(@type3,tspan,x0);

figure
plot(tsol, xsol(:,1), 'LineWidth', 3.25)
hold on
plot(tsol, xsol(:,2), 'LineWidth', 3.25)
hold on
plot(tsol, xsol(:,3), 'LineWidth', 3.25)

legend('S','E','I')
xlabel('time')
ylabel('Population')
xlim([0 150])

% - - - - - - - - - - - - - - - - - - - - - - - - - - - %
\end{lstlisting}

\noindent
To obtain figure \ref{df_gas_two_fig}(b), we use the same code but with initial conditions given by 
$\boldsymbol{(S(0), E(0), I(0)) = (10, 20, 15)}$   
\newpage

\noindent
\underline{\textbf{\large{Figure \ref{df_glb_fig}}}}\textbf{\large{ : }} The Model parameters remain the same.

\begin{lstlisting}

% - - - - - - - 3-d plot of the system - - - - - - - %

S_0 = 30;
E_0 = 10;
I_0 = 10;
x0 = [S_0 E_0 I_0];

tspan = 0 : 0.1 : 3000;
[tsol,xsol] = ode45(@type3,tspan,x0);

plot3(xsol(:,1), xsol(:,2), xsol(:,3),'LineWidth',3.25);

xlabel('Susceptible')
ylabel('Exposed')
zlabel('Infected')

xlim([0,30])
ylim([0,20])
zlim([0,15])

hold on

% -- Different Initial condition -- %
S_0 = 2.5;
E_0 = 20;
I_0 = 5;
x0 = [S_0 E_0 I_0];

tspan = 0 : 0.1 : 3000;
[tsol,xsol] = ode45(@type3,tspan,x0);

plot3(xsol(:,1), xsol(:,2), xsol(:,3),'LineWidth',3.25);

hold on

% - - - - - - - - - - - - - - - - - - - - - - - - - - - %
\end{lstlisting}
\newpage

\noindent
The same code is run for different initial conditions to obtain further trajectories of the figure \ref{df_glb_fig}. These conditions are as follows :

\begin{table}[hbt!] 
\caption{Different Initial conditions to obtain figure \ref{df_glb_fig}}
\hspace{4.5cm}
{
\begin{tabular}{|l|l|l|}
\hline
\textbf{$S(0)$} & \textbf{$E(0)$} & \textbf{$I(0)$} \\
\hline
15 & 15 & 50 \\
\hline
2.5 & 5 & 2.5 \\
\hline
30 & 5 & 2.5 \\
\hline
15 & 2 & 2 \\
\hline
15 & 1.95 & 1.95 \\
\hline
15 & 1 & 1.2 \\
\hline
16 & 0.1 & 0.1 \\
\hline
5 & 3 & 1 \\
\hline
5 & 15 & 2 \\
\hline
2 & 20 & 1 \\
\hline
\end{tabular}
}
\end{table}

\noindent
\\
Similarly, to obtain the figures \ref{inf_las_two_fig} and \ref{inf1_las_fig}, we use the parameter values given in table \ref{inf_las_parameters} whereas to obtain the figure \ref{inf3_las_fig}, we use the parameter values given in table \ref{inf3_las_parameters} with different initial conditions.

\begin{table}[hbt!] 
\caption{Different Initial conditions to obtain figure \ref{inf1_las_fig}}
\hspace{4.5cm}
{
\begin{tabular}{|l|l|l|}
\hline
\textbf{$S(0)$} & \textbf{$E(0)$} & \textbf{$I(0)$} \\
\hline
0 & 30 & 30 \\
\hline
50 & 10 & 5 \\
\hline
0 & 33 & 10 \\
\hline
0 & 32 & 22 \\
\hline
0 & 38 & 18 \\
\hline
\end{tabular}
}
\end{table}

\begin{table}[hbt!] 
\caption{Different Initial conditions to obtain figure \ref{inf3_las_fig}}
\hspace{4.5cm}
{
\begin{tabular}{|l|l|l|}
\hline
\textbf{$S(0)$} & \textbf{$E(0)$} & \textbf{$I(0)$} \\
\hline
0 & 4 & 3 \\
\hline
0 & 2 & 1 \\
\hline
2.5 & 1 & 2.6 \\
\hline
0 & 1 & 4 \\
\hline
1 & 1 & 4 \\
\hline
0 & 3 & 1 \\
\hline
\end{tabular}
}
\end{table}
\newpage

\noindent
\underline{\textbf{\large{Figure \ref{bif_fig}}}}\textbf{\large{ : }}

\begin{lstlisting}
% - - - - - -  Varying R0 by varying tetha - - - - - - %

alpha = 0.95;
beta = 0.045;
Lamda = 3;
mu = 0.05;
tetha_1 = 0.1:0.005:0.4;
eps = 0.03;
u1 = 0.1;
u2 = 0.1;
d = 0.01;
m = 0.1;
gamma = 0.01;

for i=1:length(tetha_1)
    R0(i)= (eps*beta*Lamda)/ ...
           ((mu+tetha_1(i))*(mu+eps+u1)*(mu+d+gamma));
end

% - - - - - - - - - - - - - - - - - - - - - - - - - - - %

% - - Finding disease free equilibrium for each Ro - - %

for i=1:length(R0)
    I_st_df(i) = 0;
    
    if R0(i) >1
        A = alpha*(mu+d+gamma)*(m*(mu+tetha_1(i))+beta);
        
        B = (mu+d+gamma)*(mu+tetha_1(i))*(alpha*(1-R0(i)) ...
           +(u2*(m*(mu+tetha_1(i))+beta)...
           /((mu+d+gamma)*(mu+tetha_1(i)))));
        
        C = (mu+d+gamma)*(m*(mu+tetha_1(i))+beta) ...
           + u2*(mu+tetha_1(i));
        
        D = (mu+tetha_1(i))*(mu+d+gamma)*(1-R0(i));
        
        p = [A B C D];
        I = roots(p);
        I_st(i) = I(3);
        
    else
        I_st(i) = 0;
    end       
end

[value, index] = min(abs( R0-1 ));
j=1;
for i=1:index
    RO_df(j) = R0(i);
    I_unst_df(j) = 0;
    j = j+1;
end

plot(R0, I_st,'LineWidth',1.5)
hold on
plot(R0, I_st_df,'LineWidth',1.5)
hold on
plot(RO_df,I_unst_df,)

xlabel('R_{0}')
ylabel('Infected popualtion')

% - - - - - - - - - - - - - - - - - - - - - - - - - - - %
\end{lstlisting}
\newpage

\section{Chapter 8 : Sensitivity Analysis and Heat Plots} \label{app_sen_hp}
This section includes the MATLAB codes of plots of chapter 8.

\noindent
\\
\underline{\textbf{\large{Figure \ref{sen_alpha_1}}}}\textbf{\large{ : }}

\begin{lstlisting}

% - - Sensitivity Analysis for alpha in interval I - - %

global alpha beta Lamda mu tetha eps u1 u2 d m gamma R0

alpha_vary = 0.1:0.05:0.5;
beta =  0.05;
Lamda = 2;
mu = 0.001;
tetha = 0.2;
eps = 0.03;
u1 = 0.1;
u2 = 0.1;
d = 0.01;
m = 0.1;
gamma = 0.01;

for j=1:length(alpha_vary)
    alpha = alpha_vary(j);
    R0_vary(j) = (eps*beta*Lamda)/((mu+tetha) ...
                 *(mu+eps+u1)*(mu+d+gamma));
end

% - - - - - - - - - - - - - - - - - - - - - - - - - - - %

% Plotting Infected population v/s time for each value of alpha %
 
tspan = 0 : 0.1 : 3000;
S_0 = 10;
E_0 = 20;
I_0 = 15;
x0 = [S_0 E_0 I_0];

for j = 1:length(alpha_vary)
    alpha = alpha_vary(j);
    R0 = R0_vary(j);
    [tsol,xsol] = ode45(@type3,tspan,x0);
    
    for n=1:length(xsol)
        I(n,j) = xsol(n,3);
    end
    
    plot(tsol,xsol(:,3), 'LineWidth', 3.25);
    hold on  
end

xlabel('time')
ylabel('Infective population')

xlim([0 500])
ylim([0 16])

% - - - - - - - - - - - - - - - - - - - - - - - - - - - %

% - - - - Finding the mean at each time instant - - - - %

for j=1:length(tsol)
    sum = 0;
    for n=1:length(alpha_vary)
        sum = sum + I(j,n);     
    end
    
    I_mean(j) = sum/length(alpha_vary);
  
end

figure
plot(tsol,I_mean,'LineWidth',1.5)
xlim([0 500])

xlabel('time')
ylabel('Mean Infective population')

% - - - - - - - - - - - - - - - - - - - - - - - - - - - %

% - - - - Finding the average mean square error - - - - %

for j=1:length(tsol)
    sum =0;
    for n=1:length(alpha_vary)
        mse(j,n) = (I(j,n) - I_mean(j))^2;
        sum = sum + mse(j,n);
    end
    I_error(j) = sum/length(alpha_vary);
end

figure
plot(tsol,I_error,'LineWidth',1.5)

xlabel('time')
ylabel('Mean square error')

xlim([0 500])

% - - - - - - - - - - - - - - - - - - - - - - - - - - - %
\end{lstlisting}

\noindent
\\
Similarly, the figures \ref{sen_alpha_2} to \ref{sen_u1_2} are obtained by running the same code but with the parameter values obtained from table \ref{sen_anl}.

\noindent
\\
\underline{\textbf{\large{Figure \ref{hp1}}}}\textbf{\large{ : }}

\begin{lstlisting}

% - - - - - Heat plots - varying u1 and theta  - - - - - %

global alpha beta Lamda mu tetha eps u1 u2 d m gamma 

alpha = 0.95;
beta =  0.05;
Lamda = 2;
mu = 0.001;
eps = 0.03;
u2 = 0.1;
d = 0.01;
m = 0.1;
gamma = 0.01;
tetha_vary = 0.1:0.01:1;
u1_vary = 0.1:0.01:1;

for j = 1 : length(u1_vary)
    u1 = u1_vary(j);
    
    for k = 1 : length(tetha_vary)
        tetha = tetha_vary(k);       
        R0(j,k)= (eps*beta*Lamda)/...
                 ((mu+tetha)*(mu+eps+u1)*(mu+d+gamma));
        
        if R0(j,k) < 1
            heat(j,k)=0;
   else
       A = alpha*(mu+d+gamma)*(m*(mu+tetha)+beta);
       B = (mu+d+gamma)*(mu+tetha)*(alpha*(1-R0(j,k))...
           +(u2*(m*(mu+tetha)+beta)/((mu+d+gamma)*(mu+tetha))));
       C = (mu+d+gamma)*(m*(mu+tetha)+beta) + u2*(mu+tetha);
       D = (mu+tetha)*(mu+d+gamma)*(1-R0(j,k));
            
      alpha_st = -((u2*(m*(mu+tetha)+beta))...
                 /((1-R0(j,k))*(mu+d+gamma)*(mu+tetha)));
            
       if alpha < alpha_st
           heat(j,k)= R0(j,k);
       else
           if B^2 -3*A*C <= 0
           heat(j,k)= R0(j,k);                
           else
               roots(1) = (-2*B  + (4*B^2-12*A*C)^0.5)/(6*A);
               roots(2) = (-2*B  - (4*B^2-12*A*C)^0.5)/(6*A);
                 
               f1 = A*(roots(1)^3) + B*(roots(1)^2)... 
                   + C*(roots(1)) + D;
               f2 = A*(roots(2)^3) + B*(roots(2)^2)...  
                   + C*(roots(2)) + D;
                                    
               if f1*f2 < 0
                  heat(j,k)=2;
               else
                   heat(j,k)= R0(j,k);
               end
            end
         end
      end
   end
end                   
colormap('hsv');
x=[0.01 0.1];
y=[0.1 1];
imagesc(x,y,heat);
colorbar;
xlabel({'u_{1}'})
ylabel({'\theta'})

% - - - - - - - - - - - - - - - - - - - - - - - - - - - %
\end{lstlisting}
\noindent
Similarly, the figures \ref{hp2} to \ref{hp4} are obtained by running the same code but with the parameter values obtained from table \ref{sen_anl}.
