# Supplementary material for: A Mathematical Modeling Study of COVID-19 With Reference to Immigration from Urban to Rural Population
Source: arXiv:2205.05618 source file (2022-05-06)
Supplement: Supplementary file 2 [file Appendix.tex]

\chapter{Appendix : MATLAB Codes}

In this appendix, we give the MATLAB codes for each of the figures in the thesis. 
\begin{comment}
\section{Figure \ref{df_gas_two_fig}}

\begin{lstlisting}

% --- Finding the value of R0 --- % 

global alpha beta Lamda mu tetha eps u1 u2 d m gamma R0

alpha = 0.95;
beta =  0.045;
Lamda = 2;
mu = 0.05;
tetha = 0.3;

eps = 0.03;
u1 = 0.1;
u2 = 0.1;
d = 0.01;
m = 0.1;
gamma = 0.01;

R0= (eps*beta*Lamda)/((mu+tetha)*(mu+eps+u1)*(mu+d+gamma));

\end{lstlisting}

\end{comment}
